# Supplementary material for: Exploring Parity Magnetic Effects through Experimental Simulation with Superconducting Qubits
Source: arXiv:2308.11115 source file (2023-08-22)
Supplement: Supplementary file 1 [file Supp.pdf]

# Supplemental Materials for "Exploring Parity Magnetic Effects through Experimental Simulation with Superconducting Qubits"


Yu Zhang,[1,2,*] Yan-Qing Zhu,[3,*] Jianwen Xu,[1,2,*] Wen Zheng,[1,2,†] Dong Lan,[1,2,4] Giandomenico Palumbo,[5] Nathan Goldman,[6] Shi-Liang Zhu,[7,8] Xinsheng Tan,[1,2,4,‡] Z. D. Wang,[3,§] and Yang Yu[1,2,4]

[1]*National Laboratory of Solid State Microstructures, School of Physics, Nanjing University, Nanjing 210093, China*
[2]*Shishan Laboratory, Suzhou Campus of Nanjing University, Suzhou 215000, China*
[3]*Guangdong-Hong Kong Joint Laboratory of Quantum Matter, Department of Physics, and HK Institute of Quantum Science & Technology, The University of Hong Kong, Pokfulam Road, Hong Kong, China*
[4]*Hefei National Laboratory, Hefei 230088, China*
[5]*School of Theoretical Physics, Dublin Institute for Advanced Studies, 10 Burlington Road, Dublin 4, Ireland*
[6]*Center for Nonlinear Phenomena and Complex Systems, Université Libre de Bruxelles, CP 231, Campus Plaine, B-1050 Brussels, Belgium*
[7]*Guangdong-Hong Kong Joint Laboratory of Quantum Matter, Frontier Research Institute for Physics, South China Normal University, Guangzhou 510006, China*
[8]*Guangdong Provincial Key Laboratory of Quantum Engineering and Quantum Materials, School of Physics and Telecommunication Engineering, South China Normal University, Guangzhou 510006, China*


## PARAMETERS OF THE SUPERCONDUCTING CIRCUITS

We have measured the parameters of four qubits and couplers, shown in Table. S1. We also extracted the coupling parameter, $g_{QC}/2\pi \approx 100$ MHz. In the experiments, we bias all the couplers at about $\omega_c/2\pi = 6.5$ GHz, $Q_1$ and $Q_3$ are in the higher frequency band about $\omega/2\pi = 5.7$ GHz, $Q_2$ and $Q_4$ are in the lower frequency band about $\omega/2\pi = 5.5$ GHz.

TABLE S1: Parameters of qubits and couplers

| | $Q_1$ | $Q_2$ | $Q_3$ | $Q_4$ |
|---|---|---|---|---|
| $\omega/2\pi(GHz)$ | 5.7254 | 5.5348 | 5.6716 | 5.5087 |
| $\omega/2\pi(GHz)$(sweet spot) | 6.2383 | 6.4145 | 6.2676 | 6.2168 |
| $T_1(\mu s)$ | 6.83 | 12.17 | 5.05 | 5.12 |
| $T_\phi(\mu s)$ | 0.824 | 0.806 | 0.488 | 0.366 |
| Anharmonicity(MHz) | -248.724 | -254.851 | -261.849 | -264.020 |

## PARAMETRIC MODULATION AND PHASE CALIBRATION

Firstly, we will derive all the effective couplings between two adjacent qubits. To manipulate the interaction between two qubits (take $Q_1$ and $Q_2$ for example) with complex coupling strength, not just the amplitude, we applied the flux bias $\phi_1(t) = \Phi_1 + \delta_1 \cos(\omega_{\phi_1} t + \varphi_1)$ to the coupler $C_1$, where $\Phi_1$ is the dc flux bias, $\delta_1$, $\omega_{\phi_1}$ and $\varphi_1$ is the amplitude, frequency, and phase of the sinusoidal fast-flux bias modulation, respectively. When the coupler can be adiabatically eliminated, the Lamb-shifted qubit frequency is $\tilde{\omega}_{Q_{1(2)}} = \omega_{Q_{1(2)}} + \frac{(g_{1(2),1})^2}{\Delta_{1(2),1}(\phi_1)}$ and effective coupling strength between $Q_1$ and $Q_2$ is $J_{12} = g_{12}^0 + \frac{g_{1,1}g_{2,1}}{2}(\frac{1}{\Delta_{1,1}(\phi_1)} + \frac{1}{\Delta_{2,1}(\phi_1)})$. Expanding $J_{12}$ in the parameter $\delta_1 \cos(\omega_{\phi_1} t)$ to second order, and in the rotating frame at the qubits frequencies (including the drive-induced shift), we set the frequency of the parametric modulation at $\omega_{\phi_1} = \Delta_{12,\delta_1}$ to turn on the parametrically-activated coupling and bring the excited states of qubits into resonance, where $\Delta_{12,\delta_1} = \tilde{\omega}_{Q_1} - \tilde{\omega}_{Q_2} + \frac{\delta_1^2}{4}(\frac{\partial^2 \tilde{\omega}_{Q_1}}{\partial \phi_1^2} - \frac{\partial^2 \tilde{\omega}_{Q_2}}{\partial \phi_1^2})$. Ignoring the high-order oscillation terms under rotating wave approximation, we get the effective Hamiltonian of the nearest two qubits:

$$H/\hbar = \frac{\delta_1}{2}\frac{\partial J_{12}}{\partial \phi_1}(e^{-i\varphi_1}\sigma_1^+\sigma_2^- + e^{i\varphi_1}\sigma_1^-\sigma_2^+) \tag{S1}$$

The coupling strengths in the first excited manifold can be calibrated to the same specific value by changing the parametric modulation amplitude and measuring the vacuum Rabi. While the calibration of the coupling phases is less explicit, we find that the spectrum of the system with four couplings can be used to calibrate the total phase $\varphi = \varphi_1 + \varphi_2 + \varphi_3 + \varphi_4$. We assume the coupling strengths are $\Omega$, the Hamiltonian is

$$H/\hbar = \begin{bmatrix} 0 & \Omega e^{i\varphi_1} & 0 & \Omega e^{-i\varphi_4} \\ \Omega e^{-i\varphi_1} & 0 & \Omega e^{i\varphi_2} & 0 \\ 0 & \Omega e^{-i\varphi_2} & 0 & \Omega e^{i\varphi_3} \\ \Omega e^{i\varphi_4} & 0 & \Omega e^{-i\varphi_3} & 0 \end{bmatrix} \tag{S2}$$

We have $\det(H - EI) = E^4 - 4\Omega^2 E^2 + 2\Omega^4 - 2\Omega^4 \cos(\varphi) = 0$, when $\varphi = 0$, there is one double degenerate point. When $\varphi = \pi$, there are two double degenerate points. We measure the spectrum varying with an arbitrary parametric modulation phase and find when $\varphi_3$ shifts $-2\pi/9$ the total phase can be well calibrated, as shown in Fig. S1.

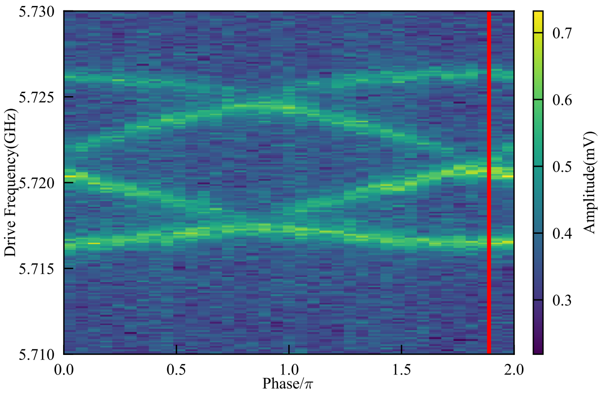


FIG. S1: Phase calibration. The energy spectrum varies with the phase of the third flux parametric modulation. The phase can be calibrated according to the number of degenerate points, as indicated by the red vertical line.

The qubit frequency is dependent on the flux threading through the SQUID of couplers, $\tilde{\omega}_{Q_1} = \omega_{Q_1} + \frac{g_{1,1}^2}{\omega_{Q_1} - \omega_{C_1}(\phi)}$. In parametric modulation, the effective qubit frequency is different from the static Lamb-shifted frequency. For simplicity, we can omit the second derivative of the frequency of the coupler to flux if the range of the parametric modulation is far detuned from the coupler's sweet spot and can be treated as linear. The frequency shift can be written as:

$$\frac{\delta_1^2}{4} \frac{\partial^2 \tilde{\omega}_{Q_1}}{\partial \phi_1^2} \approx \frac{\delta_1^2}{4} g_{1,1}^2 \frac{2}{(\omega_{Q_1} - \omega_{C_1})^3} (\frac{\partial \omega_{C_1}}{\partial \phi_1})^2 \tag{S3}$$

So the larger the effective coupling strength, the larger the drive-induced frequency shift. It is necessary to emphasize that the average of eigen-energies of the Hamiltonian tends to decrease with increasing the amplitude of parametric modulation, we measure the spectroscopy of the system with a constant pump field and calculate the undesired frequency shift at the same parameters for correction. We measure the spectrum with different parameters and constant $u(\boldsymbol{k}) = 0$, extracting the reduction of frequency as a reference, which will be compensated in later experiments and data analysis.

## AUTLER-TOWNES SPLITTING

We apply a microwave with frequency $\omega_d = \omega_{12}$ and Rabi frequency $\Omega$, there will be four dressed states in this qubit and microwave interaction system. The original first excited state $|1\rangle$ will be split into $|E_-\rangle$ and $|E_+\rangle$, whose eigen-energies respecting to $|0\rangle$ can be written as:

$$E_\pm = \omega_{01} + \Delta_{12}/2 \pm \sqrt{\Delta_{12}^2 + \Omega^2}/2 \tag{S4}$$

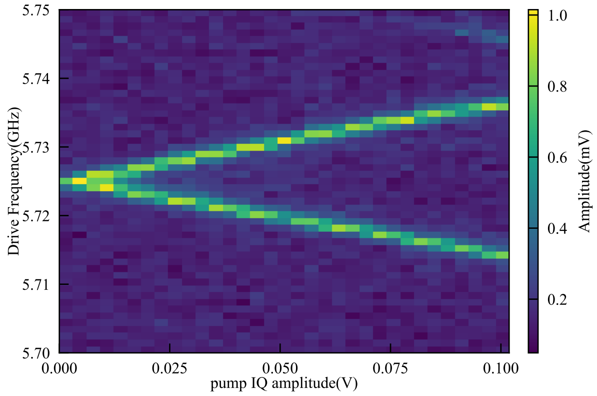


FIG. S2: Aulter-Townes splitting. Additional pump microwave field splits the first excited state $|1\rangle$ into $|E_-\rangle$ and $|E_+\rangle$. The energy gap changes linearly with the amplitude of the pump IQ signal.

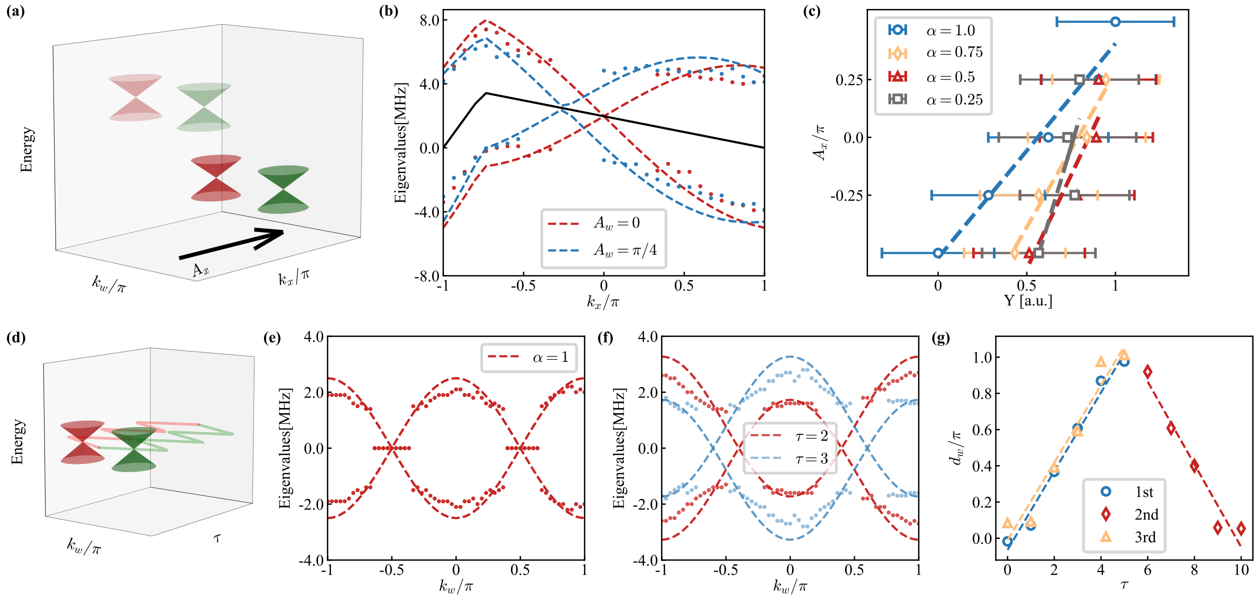


FIG. S3: Experiment results for $a = 0$. (a,b,c) represent the construction of magnetic field $B^z$. (d,e,f) show the modulation of separation of spin-1/2 monopole which can be considered as a pseudo-electric field.

we set $\Delta_{12} = 0$, the splitting equals Rabi frequency $E_+ - E_- = \Omega$, and the frequency of $|E_-\rangle$ can be tuned easily. As illustrated in Fig. S2, we vary the amplitudes of IQ input signals and measure the spectrum. From the best fit, we find that the frequency of $|E_-\rangle$ linearly depends on the pump amplitude. The relationship between the energy shift $u_0(\boldsymbol{k})$ and transversal Rabi frequency $\Omega_d/2\pi$ is $u_0(\Omega_d/2\pi)/2\pi = -0.489\Omega_d/2\pi + 7.628$ MHz. In the range $[-3\pi/4, \pi]$, the Rabi frequency of the pump microwave field changed linearly from 8.536 MHz to 15.606 MHz.

## EXPERIMENT RESULTS FOR $a = 0$

In Fig. S3, we show the magnetic field and pseudo electric field experiment results for $a = 0$ as a supplement to the text.

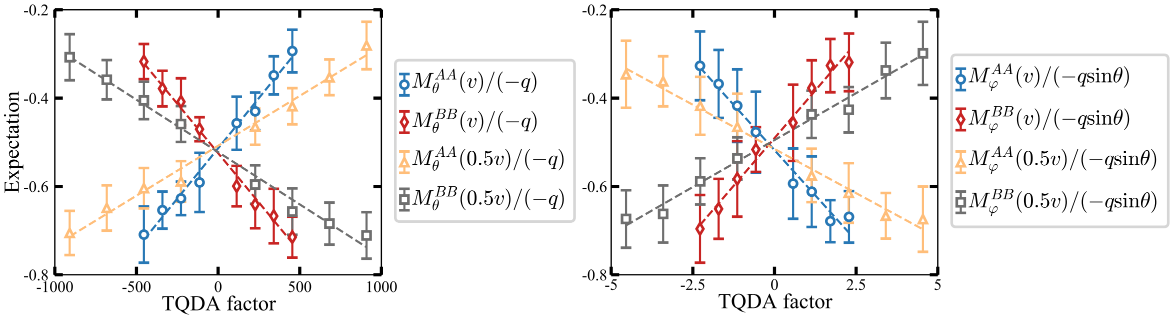


FIG. S4: TQDA. Left: The first ramp at $q = 54$ MHz. We measure the results for different initial states and ramping speeds. Expectation values change linearly with the TQDA factor. The circles represent experimental data and the dashed lines are the best fits. Right: The second ramp at $q = 6$ MHz and $\theta = 0$.

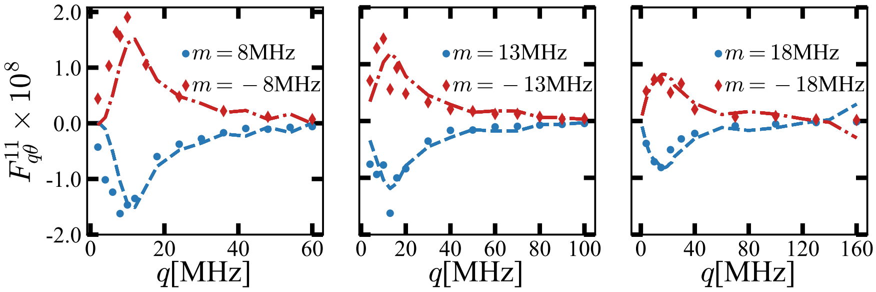


FIG. S5: According to the measurement of geometric force, calculated results of $\mathcal{F}_{q\theta}^{11}$ are illustrated for $m = \pm 8$ MHz (left), $m = \pm 13$ MHz (middle) and $m = \pm 18$ MHz (right). The dots are experiment results and the dashed lines are numerical simulations considering the decoherence.

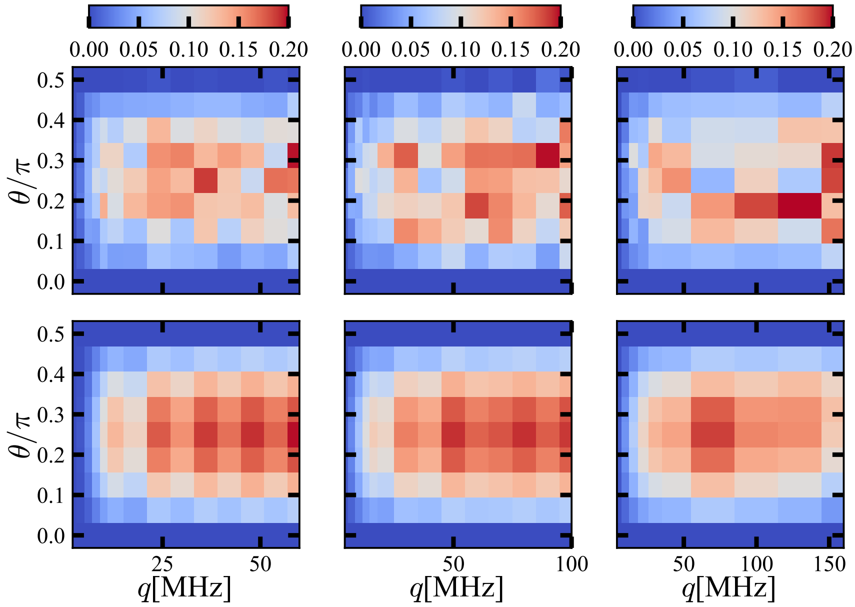


FIG. S6: Calculated results of $\mathcal{F}_{\phi\varphi}^{11}$ under the second kind of ramp for $m = 8$ MHz (left column), $m = 13$ MHz (middle column) and $m = 18$ MHz (right column). For every column, the upper panel is the experiment data, and the lower panel is the numerical simulation considering the decoherence.

## MEASUREMENT OF THE SECOND CHERN NUMBER

In the Hopf coordinates, when $(\phi,\varphi)=(0,0)$, $H_{v,\pm}$ is $H_{\phi=\varphi=0}=q\cos\theta\tilde{\Gamma}_x+q\sin\theta\tilde{\Gamma}_z+m\tilde{\Gamma}_0$. In order to reduce the inaccuracy in preparation of the initial state, we rotate the Hamiltonian so that we just need to prepare the same eigenstates at different parameters with the following unitary diagonalization.

$$H_{\mathrm{rot}}=UH_{\phi=\varphi=0}U^{\dagger} \tag{S5}$$

where $U=U_1U_2$ and $\Phi=\arccos(\frac{m}{\sqrt{q^2+m^2}})$

$$U_1=\begin{bmatrix}\cos(\frac{\Phi}{2}) & \sin(\frac{\Phi}{2}) & 0 & 0\\ -\sin(\frac{\Phi}{2}) & \cos(\frac{\Phi}{2}) & 0 & 0\\ 0 & 0 & \cos(\frac{\Phi}{2}) & -\sin(\frac{\Phi}{2})\\ 0 & 0 & \sin(\frac{\Phi}{2}) & \cos(\frac{\Phi}{2})\end{bmatrix} \tag{S6}$$

$$U_2=\begin{bmatrix}e^{\frac{i\theta}{2}} & 0 & 0 & 0\\ 0 & e^{\frac{-i\theta}{2}} & 0 & 0\\ 0 & 0 & e^{\frac{i\theta}{2}} & 0\\ 0 & 0 & 0 & e^{\frac{-i\theta}{2}}\end{bmatrix} \tag{S7}$$

In this experiment, we measure the non-adiabatic response to obtain the Berry curvature[1]. In this protocol, we slowly ramp the parameter $\mu(t)$ of the quantum system initialized at $|\Psi_i\rangle$, with a speed $v$, yielding that the generalized geometric force $M_\nu=-\langle\partial_\nu H\rangle$ with the relation $M_\nu=-\dot{\mu}\langle\mathcal{F}^{ii}_{\mu\nu}\rangle+\mathrm{const.}$. By ramping $\mu(t)$ with the speed $v/2$, we obtain the Berry curvature $\mathcal{F}^{ii}_{\mu\nu}\approx 2[M_\nu(v/2)-M_\nu(v)]/v$. This procedure is executed with four initial states $|\Psi_1\rangle=|\Psi_A\rangle$, $|\Psi_2\rangle=|\Psi_B\rangle$, $|\Psi_3\rangle=(|\Psi_A\rangle+|\Psi_B\rangle)/\sqrt{2}$ and $|\Psi_3\rangle=(|\Psi_A\rangle+i|\Psi_B\rangle)/\sqrt{2}$ where $|\Psi_A\rangle$ and $|\Psi_B\rangle$ are eigenstates of $H_{\mathrm{rot}}$, then we get the non-abelian Berry curvature as

$$\mathcal{F}_{\mu\nu}=\begin{bmatrix}\mathcal{F}^{AA}_{\mu\nu} & \mathcal{F}^{AB}_{\mu\nu}\\ (\mathcal{F}^{AB}_{\mu\nu})^* & \mathcal{F}^{BB}_{\mu\nu}\end{bmatrix}, \tag{S8}$$

where $\mathcal{F}^{AA}_{\mu\nu}=\mathcal{F}^{11}_{\mu\nu}$, $\mathcal{F}^{BB}_{\mu\nu}=\mathcal{F}^{22}_{\mu\nu}$ and $\mathcal{F}^{AB}_{\mu\nu}=2i\mathcal{F}^{33}_{\mu\nu}+2\mathcal{F}^{44}_{\mu\nu}-(1+i)(\mathcal{F}^{11}_{\mu\nu}+\mathcal{F}^{22}_{\mu\nu})$.

In this experiment, we first ramp $q(t)=q_0+v_1(t-t_m)t^2/t_m^2$ measure $M_\theta=q\sin\theta\tilde{\Gamma}_x-q\cos\theta\tilde{\Gamma}_z$ to obtain $\mathcal{F}_{q\theta}$. Similarly, $\mathcal{F}_{\phi\varphi}$ is obtained by measuring $M_\varphi=-q\sin\theta\tilde{\Gamma}_w$ with ramping $\phi(t)=\phi_0+v_2(t-t_m)t^2/t_m^2$. For different $m$, we choose different but efficient $q$s to depict the profile. For every $\theta$, we fit $\mathcal{F}(q,\theta)$ that varies with $q$ according to the analytical result, and choose $q_{\mathrm{cut}}=200$ MHz in the numerical integration. The expectation value can be quite small on account of the small perturbation term, precise measurement of the non-adiabatic response is a difficult task for practical implementation. We use the modified transitionless quantum driving algorithm (TQDA) protocol to increase the measurement signal-to-noise ratio. In the original routine, the counter-diabatic term $H_{CD}=i\sum|\partial_t n\rangle\langle n|$ is introduced to cancel the perturbation in the adiabatic process, where $|n\rangle$ is eigenstate of $H_0$. In our protocol, we design the Hamiltonian as $H=H_0+\lambda H_{CD}$, where $\lambda$ is named as the TQDA factor. We can increase the non-adiabatic response in an appropriate range, while the generalized geometric force $M_\nu$ varies linearly with $\lambda$. In practice, we set a suitable list of TQDA factors for different parameters. After the modified ramping evolution, we measure $M_\nu(\lambda)$, the observable could be amplified sufficiently and then we fit the slope $k$ of $M_\nu(\lambda)$, and extract the non-adiabatic response $M_\nu(\lambda=0)=-k$.

$$H^{CD}_{\mathrm{ramp1}}=\frac{\lambda}{2}\frac{m}{q^2(t)+m^2}\dot{q}(t)\sigma_y \tag{S9}$$

$$H^{CD}_{\mathrm{ramp2}}=\frac{-\lambda}{2}\frac{\sqrt{q^2+m^2}q\cos\theta\cos\phi(t)}{q^2+m^2+[q\cos\theta\sin\phi(t)]^2}\dot{\phi}(t)\sigma_x \tag{S10}$$

After the transformation, we just need to measure:

$$M^{\mathrm{rot}}_\theta=UM_\theta U^{\dagger}\begin{bmatrix}0 & iq & 0 & 0\\ -iq & 0 & 0 & 0\\ 0 & 0 & 0 & iq\\ 0 & 0 & -iq & 0\end{bmatrix} \tag{S11}$$

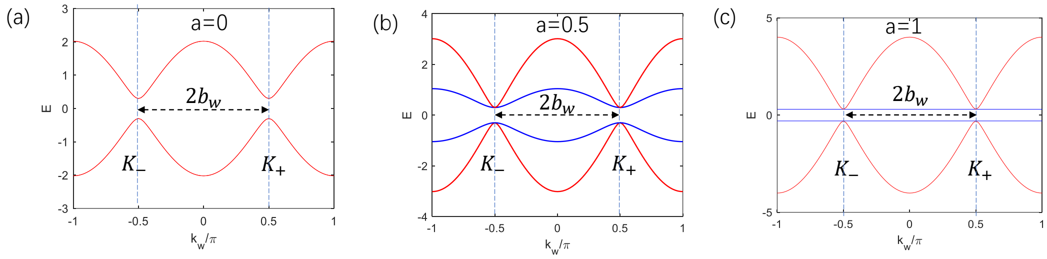


FIG. S7: Schematic of the spectrum of the gapped lattice model $H_v = H(\boldsymbol{k}) + \tilde{m}$ (a) when $a = 0$; (b)$a = 0.5$; (c)$a = 1$.

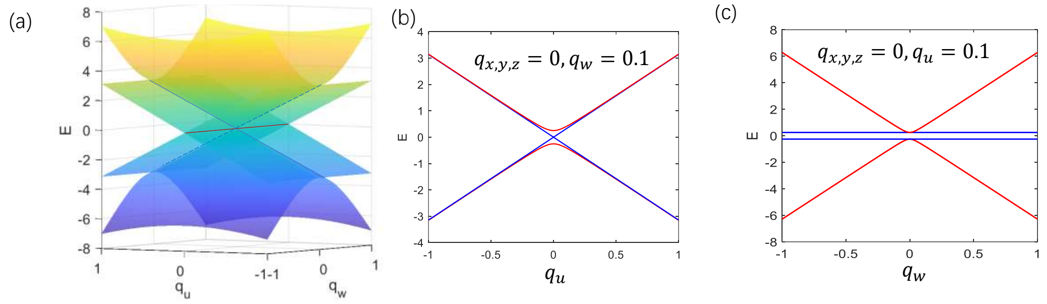


FIG. S7: 5D Nexus fermion $H_{5D}$ when $a = 1$. (a) Schematic of the spectrum when $q_x = q_y = q_z = 0$; Slice for $E$ (b) when $q_w = 0.1$; (c)$q_u = 0.1$.

$$M_\varphi^{\rm rot} = U M_\varphi U^\dagger \begin{bmatrix} 0 & 0 & -q\sin\theta & 0 \\ 0 & 0 & 0 & q\sin\theta \\ -q\sin\theta & 0 & 0 & 0 \\ 0 & q\sin\theta & 0 & 0 \end{bmatrix} \tag{S12}$$

## FRACTIONAL SECOND CHERN NUMBER FOR THE GAPPED DIRAC VALLEYS

After introducing a mass term into the 4D gapless model, we obtain a fully gapped insulator with the total Hamiltonian $H_v = H(\boldsymbol{k}) + \tilde{m}$ which hosts two Dirac-like valleys along $k_w$ direction, as shown in Fig. S7. Valley Hamiltonian near $\boldsymbol{K}_+$ ($\boldsymbol{K}_-$) is given by

$$H_{v,\pm} = q_x\tilde{\Gamma}_x + q_x\tilde{\Gamma}_x + q_z\tilde{\Gamma}_z \pm q_w\tilde{\Gamma}_w + m\tilde{\Gamma}_0. \tag{S13}$$

Each valley hosts the second Chern number is

$$\begin{aligned} C_2^\pm &= \frac{1}{32\pi^2}\int_{\mathbb{R}^4} d^4q\epsilon^{\mu\nu\alpha\beta}\ \mathrm{tr}\left(\mathcal{F}^\pm_{\mu\nu}\mathcal{F}^\pm_{\alpha\beta}\right) \\ &= \frac{1}{4\pi^2}\int_{\mathbb{R}^4} d^4q\ \mathrm{tr}\ \left(\mathcal{F}^\pm_{xy}\mathcal{F}^\pm_{zw} + \mathcal{F}^\pm_{wx}\mathcal{F}^\pm_{zy} + \mathcal{F}^\pm_{zx}\mathcal{F}^\pm_{yw}\right) \\ &= \begin{cases} \pm\frac{\mathrm{sgn}(m)}{2}, a \neq \pm 1 \\ \pm\frac{\mathrm{sgn}(m)}{8}, a = 1 \end{cases} \end{aligned} \tag{S14}$$

for $a \geq 0$. Here $\mathbb{R}^4$ denotes the full 4D real space. $\mathcal{F}^\pm_{\mu\nu}$ denotes the non-abelian Berry curvature defined for the lower two occupied bands of each valleys at $\boldsymbol{K}_+$ and $\boldsymbol{K}_-$ respectively. In fact, these two valleys hosts opposite second Chern number leading to a total zero second Chern number $C_2 = C_2^+ + C_2^- = 0$ for this phase, one could define a valley second Chern number for this model, i.e., $C_{2,v} = (C_2^+ - C_2^-)/2$.

## 5D YANG MONOPOLES AND NEXUS QUADRUPOLE NODAL POINTS

By treating $m$ as the fifth-dimensions $q_u$, we obtain a 5D model for a single nodal point. Its Hamiltonian takes the form,

$$H_{5D}(\boldsymbol{q}) = q_x\tilde{\Gamma}_x + q_y\tilde{\Gamma}_y + q_z\tilde{\Gamma}_z + q_w\tilde{\Gamma}_w + q_u\tilde{\Gamma}_0, \tag{S15}$$

where the energy spectrum

$$E = \pm\sqrt{(1\pm a)^2(q_x^2+q_y^2+q_z^2+q_w^2)+q_u^2}. \tag{S16}$$

When $a = 0$, this is a standard 5D Yang monopole [2] in momentum space whose topological charge is given by

$$Q = C_2 = \frac{1}{32\pi^2}\int_{\mathbb{S}^4} \mathrm{tr}(\mathcal{F}_{\mu\nu}\mathcal{F}_{\alpha\beta})d^4q = C_2(q_u > 0) - C_2(q_u < 0) = 1. \tag{S17}$$

In this case there is a full gap between the lower occupied and the higher empty bands except $q = 0$. Thus we can calculate the second Chern number for the lower two-fold degenerate bands on the hypersphere $\mathbb{S}^4$ enclosing the monopole. The monopole charge actually is equivalent to the difference between two massive 4D Dirac valley when taking $q_u$ as a constant. For $|a| > 0$ and $|a| \neq 1$, there is still a full gap between the lower occupied and the higher empty bands beyond the defect. The situation is similar to the case when $a = 0$ which hosts a charge $Q = 1$.

However, when $|a| = 1$, the spectrum becomes

$$E = \pm q_u, \pm\sqrt{4(q_x^2+q_y^2+q_z^2+q_w^2)+q_u^2}. \tag{S18}$$

As shown in Fig. S7, this is not a nodal point defect anymore. One could not introduce a $\mathbb{S}^4$ to fully enclose this defect with a total gapped spectrum on this surface. This is new type of Nexus fermions with four-fold degeneracy along the nodal line. The topological punctured-Chern invariant should be generalized from the 3D Nexus triple points [3] on the corresponding punctured manifold in the future.

* These authors contributed equally to this work.
† Electronic address: zhengwen@nju.edu.cn
‡ Electronic address: tanxs@nju.edu.cn
§ Electronic address: zwang@hku.hk

[S1] M. Kolodrubetz, Phys. Rev. Lett. **117**, 015301 (2016).
[S2] S. Sugawa, F. Salces-Carcoba, A. R. Perry, Y. Yue, and I. B. Spielman, Science **360**, 1429 (2018).
[S3] A. Das, E. Cornfeld, and S. Pujari, Physical Review Letters **130**, 186202 (2023).
